# Supplementary material for: Tire-road friction estimation and uncertainty assessment to improve electric aircraft braking system
Source: arXiv:2211.10336 source file (2022-11-14)
Supplement: Supplementary file 1 [file Appendix.tex]

\newpage
\clearpage
\section{Appendix}

\textcolor{red}{Appendice, solo per raccogliere figure e testo aggiuntivo da valutare}

 \begin{figure}[t]
 	\begin{center}
 		\includegraphics[width=0.8\linewidth]{img/Exp/OptimalSlipExp001.eps} 
 		\caption{Open Loop experiment. \vspace{-10pt}}
		\label{fig:openloop_old}
 	\end{center}
 \end{figure}

\begin{figure}[t]
	\begin{center}
		\includegraphics[width=0.8\linewidth]{img/Exp/OptimalSlipExp003.eps} 
		\caption{Closed Loop experiment with fixed slip set-point - SWS. \vspace{-10pt}}
		\label{fig:openloop003}
	\end{center}
\end{figure}

\begin{figure}[t]
\begin{center}
		\includegraphics[width=0.8\linewidth]{img/Exp/UncertaintyExp003.eps} 
		\caption{Closed Loop experiment -SWS - Uncertainty. \vspace{-10pt}}
		\label{fig:closedloop003-uncertainty}
\end{center}
\end{figure}

\begin{figure}[t]
	\begin{center}
		\includegraphics[width=0.8\linewidth]{img/Exp/OptimalSlipExp004.eps} 
		\caption{Closed Loop experiment with set point given by the MLP estimated best slip - SWS. \vspace{-10pt}}
		\label{fig:closedloop004}
	\end{center}
\end{figure}

\begin{figure}[t]
\begin{center}
		\includegraphics[width=0.8\linewidth]{img/Exp/UncertaintyExp004.eps} 
		\caption{Closed Loop experiment with set point given by the MLP estimated best slip - SWS - Uncertainty. \vspace{-10pt}}
		\label{fig:closedloop004-uncertainty}
\end{center}
\end{figure}

The results for the closed loop case, SWs sequence of transitions, are reported in the Figure \ref{fig:closedloop007} for the fixed slip set-point and in the Figures \ref{fig:closedloop008} and \ref{fig:closedloop008-uncertainty} for set point given the MLP best slip estimate.

\begin{figure}[t]
	\begin{center}
		\includegraphics[width=0.8\linewidth]{img/Exp/OptimalSlipExp007.eps} 
		\caption{Closed Loop experiment with fixed slip set-point - DSD. \vspace{-10pt}}
		\label{fig:closedloop007}
	\end{center}
\end{figure}

\begin{figure}[t]
\begin{center}
		\includegraphics[width=0.8\linewidth]{img/Exp/OptimalSlipExp008.eps} 
		\caption{Closed Loop experiment with set point given by the MLP estimated best slip - DSD. \vspace{-10pt}}
		\label{fig:closedloop008}
\end{center}
\end{figure}

\begin{figure}[t]
\begin{center}
		\includegraphics[width=0.8\linewidth]{img/Exp/UncertaintyExp008.eps} 
		\caption{Closed Loop experiment with set point given by the MLP estimated best slip - DSD. \vspace{-10pt}}
		\label{fig:closedloop008-uncertainty}
\end{center}
\end{figure}

 \begin{figure}[t]
 \begin{center}
 		\includegraphics[width=0.8\linewidth]{img/Exp/UncertaintyExp001.eps} 
 		\caption{Open Loop experiment - uncertainty vs slip. \vspace{-10pt}}
 		\label{fig:openloop001-uncertainty}
 \end{center}
\end{figure}

\begin{figure}[t]
\begin{center}
		\includegraphics[width=0.8\linewidth]{img/Exp/OptimalSlip_subplotExp003.eps} 
		\caption{Closed Loop experiment 003 \vspace{-10pt}}
%		\label{fig-app:openloop001-uncertainty}
\end{center}
\end{figure}

\begin{figure}[t]
\begin{center}
		\includegraphics[width=0.8\linewidth]{img/Exp/OptimalSlipExp003.eps} 
		\caption{Closed Loop experiment 003 \vspace{-10pt}}
%		\label{fig-app:openloop001-uncertainty}
\end{center}
\end{figure}

\begin{figure}[t]
\begin{center}
		\includegraphics[width=0.8\linewidth]{img/Exp/SlipMuExp003.eps} 
		\caption{Closed Loop experiment 003 \vspace{-10pt}}
%		\label{fig-app:openloop001-uncertainty}
\end{center}
\end{figure}

\begin{figure}[t]
\begin{center}
		\includegraphics[width=0.8\linewidth]{img/Exp/UncertaintyExp003.eps} 
		\caption{Closed Loop experiment 003 \vspace{-10pt}}
%		\label{fig-app:openloop001-uncertainty}
\end{center}
\end{figure}

%%%%%%%%%%

% 004
\begin{figure}[t]
\begin{center}
		\includegraphics[width=0.8\linewidth]{img/Exp/OptimalSlip_subplotExp004.eps} 
		\caption{Closed Loop experiment 004 \vspace{-10pt}}
%		\label{fig-app:openloop001-uncertainty}
\end{center}
\end{figure}

\begin{figure}[t]
\begin{center}
		\includegraphics[width=0.8\linewidth]{img/Exp/OptimalSlipExp004.eps} 
		\caption{Closed Loop experiment 004 \vspace{-10pt}}
%		\label{fig-app:openloop001-uncertainty}
\end{center}
\end{figure}

\begin{figure}[t]
\begin{center}
		\includegraphics[width=0.8\linewidth]{img/Exp/SlipMuExp004.eps} 
		\caption{Closed Loop experiment 004 \vspace{-10pt}}
%		\label{fig-app:openloop001-uncertainty}
\end{center}
\end{figure}

\begin{figure}[t]
\begin{center}
		\includegraphics[width=0.8\linewidth]{img/Exp/UncertaintyExp004.eps} 
		\caption{Closed Loop experiment 004 \vspace{-10pt}}
%		\label{fig-app:openloop001-uncertainty}
\end{center}
\end{figure}

%%%%%%%%%%

% 005
\begin{figure}[t]
\begin{center}
		\includegraphics[width=0.8\linewidth]{img/Exp/OptimalSlip_subplotExp005.eps} 
		\caption{Closed Loop experiment 005 \vspace{-10pt}}
%		\label{fig-app:openloop001-uncertainty}
\end{center}
\end{figure}

\begin{figure}[t]
\begin{center}
		\includegraphics[width=0.8\linewidth]{img/Exp/OptimalSlipExp005.eps} 
		\caption{Closed Loop experiment 005 \vspace{-10pt}}
%		\label{fig-app:openloop001-uncertainty}
\end{center}
\end{figure}

\begin{figure}[t]
\begin{center}
		\includegraphics[width=0.8\linewidth]{img/Exp/SlipMuExp005.eps} 
		\caption{Closed Loop experiment 005 \vspace{-10pt}}
%		\label{fig-app:openloop001-uncertainty}
\end{center}
\end{figure}

\begin{figure}[t]
\begin{center}
		\includegraphics[width=0.8\linewidth]{img/Exp/UncertaintyExp005.eps} 
		\caption{Closed Loop experiment 005 \vspace{-10pt}}
%		\label{fig-app:openloop001-uncertainty}
\end{center}
\end{figure}

%%%%%%%%%%

% 006
\begin{figure}[t]
\begin{center}
		\includegraphics[width=0.8\linewidth]{img/Exp/OptimalSlip_subplotExp006.eps} 
		\caption{Closed Loop experiment 006 \vspace{-10pt}}
%		\label{fig-app:openloop001-uncertainty}
\end{center}
\end{figure}

\begin{figure}[t]
\begin{center}
		\includegraphics[width=0.8\linewidth]{img/Exp/OptimalSlipExp006.eps} 
		\caption{Closed Loop experiment 006 \vspace{-10pt}}
%		\label{fig-app:openloop001-uncertainty}
\end{center}
\end{figure}

\begin{figure}[t]
\begin{center}
		\includegraphics[width=0.8\linewidth]{img/Exp/SlipMuExp006.eps} 
		\caption{Closed Loop experiment 006 \vspace{-10pt}}
%		\label{fig-app:openloop001-uncertainty}
\end{center}
\end{figure}

\begin{figure}[t]
\begin{center}
		\includegraphics[width=0.8\linewidth]{img/Exp/UncertaintyExp006.eps} 
		\caption{Closed Loop experiment 006 \vspace{-10pt}}
%		\label{fig-app:openloop001-uncertainty}
\end{center}
\end{figure}

%%%%%%%%%%

% 006
\begin{figure}[t]
\begin{center}
		\includegraphics[width=0.8\linewidth]{img/Exp/OptimalSlip_subplotExp007.eps} 
		\caption{Closed Loop experiment 007 \vspace{-10pt}}
%		\label{fig-app:openloop001-uncertainty}
\end{center}
\end{figure}

\begin{figure}[t]
\begin{center}
		\includegraphics[width=0.8\linewidth]{img/Exp/OptimalSlipExp007.eps} 
		\caption{Closed Loop experiment 007 \vspace{-10pt}}
%		\label{fig-app:openloop001-uncertainty}
\end{center}
\end{figure}

\begin{figure}[t]
\begin{center}
		\includegraphics[width=0.8\linewidth]{img/Exp/SlipMuExp007.eps} 
		\caption{Closed Loop experiment 007 \vspace{-10pt}}
%		\label{fig-app:openloop001-uncertainty}
\end{center}
\end{figure}

\begin{figure}[t]
\begin{center}
		\includegraphics[width=0.8\linewidth]{img/Exp/UncertaintyExp007.eps} 
		\caption{Closed Loop experiment 007 \vspace{-10pt}}
%		\label{fig-app:openloop001-uncertainty}
\end{center}
\end{figure}

%%%%%%%%%%

% 008
\begin{figure}[t]
\begin{center}
		\includegraphics[width=0.8\linewidth]{img/Exp/OptimalSlip_subplotExp008.eps} 
		\caption{Closed Loop experiment 008 \vspace{-10pt}}
%		\label{fig-app:openloop001-uncertainty}
\end{center}
\end{figure}

\begin{figure}[t]
\begin{center}
		\includegraphics[width=0.8\linewidth]{img/Exp/OptimalSlipExp008.eps} 
		\caption{Closed Loop experiment 008 \vspace{-10pt}}
%		\label{fig-app:openloop001-uncertainty}
\end{center}
\end{figure}

\begin{figure}[t]
\begin{center}
		\includegraphics[width=0.8\linewidth]{img/Exp/SlipMuExp008.eps} 
		\caption{Closed Loop experiment 008 \vspace{-10pt}}
%		\label{fig-app:openloop001-uncertainty}
\end{center}
\end{figure}

\begin{figure}[t]
\begin{center}
		\includegraphics[width=0.8\linewidth]{img/Exp/UncertaintyExp008.eps} 
		\caption{Closed Loop experiment 008 \vspace{-10pt}}
%		\label{fig-app:openloop001-uncertainty}
\end{center}
\end{figure}
